# Supplementary material for: CliniQG4QA: Generating Diverse Questions for Domain Adaptation of Clinical Question Answering
Source: arXiv:2010.16021 source file (2021-12-11)
Supplement: Supplementary file 1 [file 7_Appendix.tex]

\section{Post-Processing of Extracted Answer Evidences}
\label{apx:extract_evidence}
This section is dedicated to the discussion of heuristic rules developed to improve the quality of the extracted answer evidence.

We observe that when we directly apply the ClinicalBERT \cite{alsentzer2019publicly} system described in Section 3.2 (in the main content) on clinical texts, the extracted answer evidences sometimes are broken sentences due to the noisy nature and uninformative language (e.g., acronyms) of clinical texts. To make sure the extracted evidences are meaningful, we designed a \textit{``merge-and-drop''} heuristic rule to further improve the extractor’s accuracy. Specifically, for each extracted evidence candidate, we first examine the \textit{length}  (number of tokens) of the extracted evidence. If the length is larger than the threshold $\eta$, we keep this evidence; otherwise, we compute the \textit{distance}, i.e., the number of tokens between the current candidate span and the closest span. If the \textit{distance} is smaller than the threshold $\gamma$, we merge these two ``close-sitting'' spans; otherwise, we drop this over-short evidence span. In our experiments, we set $\eta$ and $\gamma$ to be 3 and 3, respectively, since they help the QA system achieve the best performance on the dev set

The intuitions behind this heuristic rule are listed as follows: 1) we should discard as few useful answer evidence spans as possible, so we first resort to merging before simply dropping a span; 2) Commonly, if two spans (and at least one is a short span) are sitting close to each other, they should have been recognized as a single answer evidence. For example, the \texttt{BIO} label of a snippet ``chief complaint: altered mental status major'' is predicted as ``B O B I I O'', whereas, a clinical expert will label it as ``B I I I I O''. However, if they sit far away, merging would introduce noisy information; 3) long spans are always more informative and contain less misleading information compared with short spans (e.g., ``the patient had left leg pain'' v.s. ``pain'').

\section{Implementation Details}
\label{apx:implementation_details}
We provide very detailed implementation details to foster reproducibility. 

\begin{table}[t]
\centering
\begin{tabular}{lcc}
\hline
 & QPP acc & QG acc \\ \hline
NQG & / & 74.32 \\
NQG++ & / & 74.54 \\
BERT-SQG & / & 79.78 \\ \hline
QPP-NQG & 99.2 & 85.15 \\
QPP-NQG++ & 99.17 & 85.27 \\
QPP-BERT-SQG & 99.19 & 88.15 \\ \hline
\end{tabular}
\caption{QPP and QG performance on dev set in terms of per-token accuracy. All numbers are percentages.}
\label{dev_qg}
\end{table}
\begin{table}[t]
\centering
\resizebox{\linewidth}{!}{
\begin{tabular}{lccc}
\hline
\model & QG & QA & overall \\ \hline
NQG\&DocReader & 6 & 17 & 24.5 \\
NQG++\&DocReader & 7.5 & 20 & 29 \\
BERT-SQG\&DocReader & 13 & 18 & 32.5 \\
NQG\&CliniBERT & 6 & 3.5 & 11 \\
NQG++\&CliniBERT & 7.5 & 4 & 13 \\
BERT-SQG\&CliniBERT & 13.5 & 3.5 & 18.5 \\ \hline
\end{tabular}}
\caption{The running time (hour) of QPP-augmented QG, QA and overall \model based on our selected QG \& QA combinations}
\label{run_time}
\end{table}
\begin{table}[t]
\centering
\begin{tabular}{lcc}
\hline
Parameter & Search Trials & Best \\ \hline
Dropout & {[}0.3,0.45,0.6,0.75,0.9{]} & 0.75 \\
LSTM Layers & {[}1,2,3,4{]} & 3 \\
QP Length & {[}1,2,3{]} & 2 \\ \hline
\end{tabular}
\caption{Hyperparameter searches for Question Phrase Prediction (QPP) Module}
\label{QPP_tune}
\end{table}

\begin{table}[t]
\centering
\begin{tabular}{lcc}
\hline
Parameter & Search Trials & Best \\ \hline
length ($\eta$) & {[}1,3,5,10{]} & 3 \\
distance ($\gamma$) & {[}1,3,5,10{]} & 3 \\ \hline
\end{tabular}
\caption{Hyperparameter searches for \textit{``merge-and-drop"} method}
\label{AEE_tune}
\end{table}
\subsection{Prepossessing}
\subsubsection{Dataset Prepossessing}
\textbf{emrQA}\footnote{https://github.com/panushri25/emrQA} We prune the emrQA set by removing QA pairs whose question is an indicator (e.g., ``meds'') so that all remaining QA pairs contain valid questions. We also leverage SciSpacy\footnote{https://allenai.github.io/scispacy/}, a package containing spaCy models for processing clinical text, to do tokenization in order for the trained QG models to have a better understanding over clinical notes.

\noindent\textbf{MIMIC-III}\footnote{ https://mimic.physionet.org/gettingstarted/access/} Similarly, we also leverage SciSpacy to do tokenization.

\subsubsection{Question Phrases Identification}
\label{apx:QPP_I}
In order to utilize our Question Phrase Prediction (QPP) module and make our QPP module generic enough without loss of generality, we identify valid n-gram Question Phrases in an automatic way.

To prepare an exhaustive list of valid n-gram Question Phrases, we first collect all of the first \textit{n} words appearing in Ground Truth Questions in emrQA, forming three (i.e., \textit{n}=1, 2, 3) raw Question Phrases set.

We observe that all uni-grams are valid question phrases (e.g., ``How'', ``When'', ``What''), so we don't do any pruning and keep the uni-gram question phrases set as it is.

As for n-gram (n $\geq$ 2) Question Phrases set, we conduct fine-grained filtering. We only consider n-grams with occurrence frequency greater than the threshold $\zeta$ as valid n-gram Question Phrases. In our experiment, we set $\zeta$ as 0.02\%. Less frequent n-gram words (i.e., frequency $<$ 0.02\%) will degrade to unigram Question Phrases in accordance with corresponding question types (e.g., ``Has lasix'' $\rightarrow$ ``Has''*) so as to maintain lossless. In the end, n-gram (n $\geq$ 2) Question Phrases sets, without any information loss, are consisting of both n-gram Question Phrases and degraded unigram Question Phrases.

\subsection{Models Implementation}
\label{sec:implementation}
\textbf{Base QA \& QG Models} We re-implement the three base QG models using Pytorch and have ensured that they achieve comparable performance as originally reported. The best QG model is selected using the per-token accuracy of both the QPP module (if applicable) and QG on dev set, and dev results are listed in Table \ref{dev_qg}.

For QA models, we used their open-sourced implementation.\footnote{DocReader: https://github.com/facebookresearch/DrQA. ClinicalBERT: https://github.com/EmilyAlsentzer/clinicalBERT.} The best QA model is selected using EM and F1 on dev set, and dev results are also included in Table 3 (in the main content). 
Hyperparameters of QG models are set to be the same as in the original paper and hyperparameters of QA models are set according to the guidance of \cite{yue2020CliniRC}.

\begin{table*}[t!]
\centering
\caption{Distributions of the generated questions of different models and the ground truth in the emrQA dataset. QPP: Question Phrase Prediction; KL: Kullback–Leibler divergence. All numbers are percentages.}
\resizebox{\linewidth}{!}{%
\begin{tabular}{lccccccccccc|c}
\hline
Models & \textbf{What} & \textbf{When} & \textbf{Has} & \textbf{Was} & \textbf{Why} & \textbf{How} & \textbf{Is} & \textbf{Did} & \textbf{Can} & \textbf{Any} & \textbf{Does} &  \textbf{\begin{tabular}[c]{@{}c@{}}KL\\ (Gen$||$GT)\end{tabular}} \\ \hline
NQG & 0.00 & 0.00 & 3.95 & 0.00 & 0.00 & 0.00 & 0.00 & 0.00 & 0.00 & 0.00 & 96.05 & 84.2 \\
+BeamSearch & 29.94 & 0.00 & 5.54 & 0.00 & 0.00 & 0.00 & 1.38 & 0.00 & 0.00 & 0.00 & 63.14 & 45.2 \\
\textbf{+QPP (Ours)} & 8.39 & 0.01 & 25.37 & 4.44 & 0.91 & 0.87 & 9.09 & 0.27 & 4.03 & 12.72 & 33.89 & \textbf{11.0} \\ \hline
NQG++ & 0.09 & 0.00 & 3.53 & 0.00 & 0.00 & 0.10 & 0.00 & 0.00 & 0.00 & 0.00 & 96.28 & 84.3 \\
+BeamSearch & 44.04 & 0.00 & 0.09 & 0.00 & 0.00 & 0.22 & 2.01 & 0.00 & 0.00 & 0.00 & 53.64 & 66.4 \\
\textbf{+QPP (Ours)} & 8.09 & 0.01 & 25.54 & 4.42 & 0.75 & 0.81 & 9.16 & 0.23 & 4.05 & 12.80 & 34.13 & \textbf{11.2} \\ \hline
BERT-SQG & 0.72 & 0.00 & 6.32 & 0.00 & 0.00 & 0.00 & 0.00 & 0.00 & 0.00 & 0.00 & 92.96 & 74.5 \\
+BeamSearch & 29.31 & 0.00 & 0.03 & 0.00 & 0.00 & 0.00 & 25.05 & 0.00 & 0.00 & 0.00 & 45.62 & 47.4  \\
\textbf{+QPP (Ours)} & 8.01 & 0.01 & 25.56 & 4.44 & 0.82 & 0.80 & 9.17 & 0.25 & 4.05 & 12.74 & 34.16 & \textbf{11.2} \\ \hline
GT & 13.80 & 0.01 & 26.73 & 1.94 & 0.63 & 1.16 & 13.24 & 0.14 & 1.31 & 4.11 & 36.93 & - \\ \hline
\end{tabular}%
}
\vspace{-10pt}
\label{tbl:ques_distribution}
\end{table*}

\noindent\textbf{Question Phrase Prediction (QPP) Module.} Word embeddings are initialized by Glove 300d vectors\footnote{http://nlp.stanford.edu/data/glove.840B.300d.zip}. We adopt a feature-rich Encoder\footnote{Lexical features are extracted by \cite{neumann2019scispacy}} to effectively encode Clinical lexical information. We set the LSTM hidden unit size to 600 and set the number of layers of LSTMs to 3 in both encoder and decoder. Optimization is performed using stochastic gradient descent (SGD) for 20 epochs, with an initial learning rate of 1.0. After each epoch, we evaluate the per-label accuracy on the dev set. If the accuracy does not improve, we halve the learning rate. The mini-batch size is set at 128. Dropout with probability 0.75 is applied between vertical LSTM layers. The gradient is clipped when its norm exceeds 5. Besides, we set the length of a question phrase $l$ to 2, which gives the best performance on validation. The total number of parameters is around 17M under our best-performing setting.

\noindent\textbf{Answer Evidence Extractor.} We fine-tune a ClinicalBERT model in Named Entity Recognition (NER) fashion using \texttt{BIO} tagging scheme\footnote{https://github.com/huggingface/transformers/tree/master/ examples/token-classification}. When conducting fine-tuning on our QG train set, we set max length, batch size, number of epochs, and random seed to be 510, 16, 20 and 6, respectively. We adopt the official NER evaluation script\footnote{http://deeplearning.net/tutorial/code/conlleval.pl} to do the evaluation on QG dev set, and obtained 80.17 F1 score. We then deployed this system to extract raw answer evidence spans. After raw extraction, we utilized our own heuristic rules (i.e., \textit{``merge-and-drop''}) to further polish the raw spans as described in Appendix \ref{apx:extract_evidence}. 

\noindent\textbf{Multi-Label Classification (MLC) Comparison.} We implement Binary Relevance (BR) and Classifier Chain (CC) by means of Scikit-Multilearn \cite{2017scikit}, an open-source library for the MLC task. 

\noindent\textbf{Computational Resources.} All experiments are conducted using one single GeForce GTX 2080 Ti 12 GB GPU (with significant CPU resources). We train the QPP module and QG model together though they can be trained separately. The overall running time of our \model system depends on the particular QG and QA models adopted. For our selected QG and QA models, the approximated overall running time of \model is listed in Table \ref{run_time}. However, training a QPP module separately is fast, which only takes less than 1 hour with the current setting. Meanwhile, the running time of our Answer Evidence Extractor roughly takes 1.5 hours on average. 

\subsection{Hyperparameter Search}
In order to have a best-performing Question Phrase Prediction (QPP) module, we manually tuned the hyperparameters listed in Table \ref{QPP_tune}. The hyperparameters are tuned on QG dev set using Relevance and Diversity Metrics listed in Section 4.3 (in the main content). 

\noindent In order to have a best-performing post-processing method (i.e., \textit{``merge-and-drop''}) in Answer Evidence Extraction module, we manually tuned the hyperparameters listed in Table \ref{AEE_tune}. The hyperparameters are tuned on the QA dev set using Exact Match (EM) and F1. 

\section{Distributions of Generated Questions of Different QG Models }
The detailed distributions of the generated questions of different models and the ground truth in emrQA dataset are listed in table \ref{tbl:ques_distribution}.

% \section{Impact of Question Phrase Length}
% As shown in Table \ref{tbl:ablation}, when question phrase length is set at 2, the model achieves the best performance overall. Therefore, we set the length at 2, which allows the model to generate both relevant and diverse questions as well as have a smaller search space. 
% \input{Tables/table4}

% \input{Tables/tableA6}
